# Supplementary material for: Online Dating Recommendations: Matching Markets and Learning Preferences
Source: arXiv:1401.8042 source file (2014-01-31)
Supplement: Supplementary file 1 [file appendix.tex]

\section{Conditional Entropy and Mutual Information}
The conditional entropy of a discrete random variable $X$ given $Y$, denoted as $H(X|Y)$, measure the required information to describe the outcome of $X$ given $Y$ is known. It is defined as:
\begin{align*}
H(X|Y) &= \sum_{y}P(y)H(X|Y=y) \\
			&= \sum_y\left( P(y)\sum_xP(x|y)\log\frac{1}{P(x|y)}\right) \\
			&= \sum_x\sum_yP(x,y)\log\frac{P(x)}{P(x,y)}
\end{align*}
where $P(x)=P(X=x),P(y)=P(Y=y)$ and $P(x,y)=P(X=x,Y=y)$.

The Mutual Information of two random variable $X$ and $Y$, denoted as $I(X;Y)$, describes the mutual dependency of the two variables. The larger the mutual information is, the more information the two variables share. It is defined as:
\begin{align*}
I(X;Y) 	&= \sum_x\sum_yP(x,y)\log\left(\frac{P(x,y)}{P(x)P(y)}\right) 
\end{align*}

\section{Information Gain Ratio}
\textbf{Information} We use entropy as the information to determine a random variable. In our model, this variable is \textit{``reply''}.  Let $n_y$ be the number of messages replied by receivers in a data set, $n_n$ be the number of non-replied messages, the information required to predict a receiver's reply as$$\text{Info}(n_y, n_n)=H(\text{``reply''})=-\frac{n_y}{n_y+n_n}\log \frac{n_y}{n_y+n_n} -\frac{n_n}{n_y+n_n}\log \frac{n_n}{n_y+n_n}$$

\textbf{Information Given a Feature} Suppose a feature $f$ of $V$ values divides a data set into $V$ subsets, the $v$-th subset contains $n_y^{(v)}$ relied messages and $n_n^{(v)}$ non-replied ones. We define the information required to determine \textit{``reply''} given this feature as  $$In(f;reply) = \text{Info}_f([n_y^{(1)},n_n^{(1)}], [n_y^{(2)},n_n^{(2)}], \cdots, [n_y^{(V)},n_n^{(V)}]) = \sum_{v=1}^{V}\frac{n_y^{(v)}+n_n^{(v)}}{\sum_{j=1}^{V}(n_y^{(j)}+n_n^{(j)})}\text{Info}(n_y^{(v)},n_n^{(v)})$$

\textbf{Information Gain Ratio of a Feature}
Information Gain about the random variable \textit{``reply''} from the observation of a random variable $f$ represents the information provided by $f$ to determine  \textit{``reply''}. The formula is $IG(f;``reply'') = \text{Info}(n_y,n_y)-In(f;``reply'')$. Since Information Gain bias with high score towards a feature with a large number of possible values, we use Information Gain Ratio to measure a features information by computing $$IGR(f;``reply'') = \frac{IG(f;``reply'')}{\text{Info}(n_y^{(1)}+n_n^{(1)}, n_y^{(2)}+n_n^{(2)}, \cdots, n_y^{(V)}+n_n^{(V)})}$$  
where $\text{Info}(n_y^{(1)}+n_n^{(1)}, n_y^{(2)}+n_n^{(2)}, \cdots, n_y^{(V)}+n_n^{(V)})$ is the entropy of the size of $f$'s possible values. If a feature $f$ has high information gain about \textit{``reply''}, the information gain ratio tends to be large. But if it has a large size of possible values, the information gain ratio will be small.
